# Supplementary material for: Atomic-scale compensation phenomena at polar interfaces
Source: arXiv:1010.5517 source file (2010-10-26)
Supplement: Supplementary file 1 [file Supplemental_materials.pdf]

Supplemental materials

# Atomic-scale compensation phenomena at polar interfaces

Matthew F. Chisholm[1*], Weidong Luo[2,1], Mark P. Oxley [2,1], Sokrates T. Pantelides[2,1], Ho Nyung Lee[1]

[1]*Materials Science and Technology Division, Oak Ridge National Laboratory, Oak Ridge, Tennessee 37831, USA*

[2]Department of Physics and Astronomy, Vanderbilt University, Nashville, Tennessee 37235, USA

The films used in this investigation were grown by pulsed laser deposition. A KrF excimer laser with a wavelength of 248 nm was used to ablate ceramic PZT target material onto the substrate held at 625˚C in 100 mTorr of $O_2$. The PZT films were deposited directly onto STO and onto SRO films that were grown at 700˚C in 100 mTorr on $SrTiO_3$. X-ray diffraction independently confirmed that the PZT films were fully strained, exhibiting the coherent in-plane lattice dimensions of STO, which corresponds to 1.2 % lattice strain in the PZT films. The typical polarization of our PZT films exceeds 80 μC/cm$^2$, which is amongst the highest polarization values from PZT.

The two interfaces were examined in cross section with an aberration-corrected 300 kV STEM and a collector angle of 10 mrad. Cross sections of both interfaces were prepared using a combination of mechanical polishing and ion milling. Careful mechanical polishing minimized the amount of ion milling done with 3 keV Ar ions. Final milling was done using a 0.5 keV beam. High-quality dark-field and bright-field images were

collected simultaneously combining the direct interpretability of the Z-contrast image with the much greater contrast variations possible in phase contrast imaging [1]. Fig. S1 is a simultaneously collected HAADF and BF image pair showing the <110> projection of the PZT/STO interfacial region. The Z-contrast image clearly reveals the columns of the large atomic number elements and, thus, the interface between the Pb-containing film and the less intense Sr-containing substrate. The imaging conditions have been tuned so that the phase-contrast image reveals the oxygen column positions that are very difficult to see in the Z-contrast image. The Z-contrast image is used both as a structural reference and as evidence that the simultaneously recorded phase-contrast image can be directly interpreted. At these imaging conditions the atomic column positions in the phase-contrast image are dark. The image contrast is typically inverted to facilitate automatic image feature identification.

STEM BF image simulations of PTO as viewed in the <100> projection were carried out using a Bloch wave method [2]. A detector semi-angle of 10 mrad was used with a probe forming semi-angle of 23 mrad. Spherical aberration of $C_s$=-0.037 and $C_5$=100 mm were used in the simulations. A thickness of 7 nm and a defocus of -6 nm were selected to give black atom contrast consistent with the experimental observations. This contrast may be achieved for a number of different thickness/defocus settings. Fig. S2 shows a montage of simulated images with ± 5mrad of crystal tilt in the [100] and [010] directions simulating the effect of mis-tilt of the sample during imaging. These tilts produce a consistent shifting of apparent column locations in the direction of the tilt by approximately 0.1 Å. However, there is no discernable shift in the relative positions of the Pb and O columns, which is the experimentally measured quantity.

Fig. S3 shows a 180˚ domain wall seen in the PZT film grown on the thin SRO layer. Marking the oxygen positions in red and Ti positions in green, the two domains and the 1nm thick domain wall are revealed. All the 180 degree domain walls imaged in this study show a transition of polarization from up to down over about 4 PbO planes.

While we believe that the superlattice calculations described in the text best reproduce the interfaces in relatively thick ferroelectric films on substrates, we have also carried out similar calculations on single PTO/STO slabs with free surfaces with $TiO_2$ termination. The atomic positions in the bottom STO layer were fixed to the bulk STO positions to simulate the STO substrate, while the rest of the STO and PTO layers were relaxed. The ferroelectric displacements in the interfacial region of the PTO are severely suppressed as shown in Fig. 4(a). The remaining polarization is small and points towards the STO substrate, contrary to our experimental observation. When an O vacancy is introduced in the PbO layer at the interface, as shown in Fig. 4(b), the displacements in PTO are recovered. The polarization points towards the surface, in agreement with experiment.

One might surmise that, by controlling the concentration of oxygen vacancies during the deposition process, it would be possible to optimize ferroelectric properties. More specifically, growing or annealing the samples at high oxygen pressure should suppress ferroelectricity or force compensation by another mechanism. We note, however, that the present samples were grown at 100 mTorr of oxygen, which is relatively high partial pressure. We infer that, even under such pressure, oxygen vacancies are incorporated in

the interfacial region because of a large energy gain arising from the stabilization of the ferroelectric state.

References

[1] Y. N. Chang *et al.*, Phys. Rev. Lett. **103**, 057201 (2009).

[2] L. J. Allen *et al.*, Ultramicroscopy, **96**, 47 (2003).

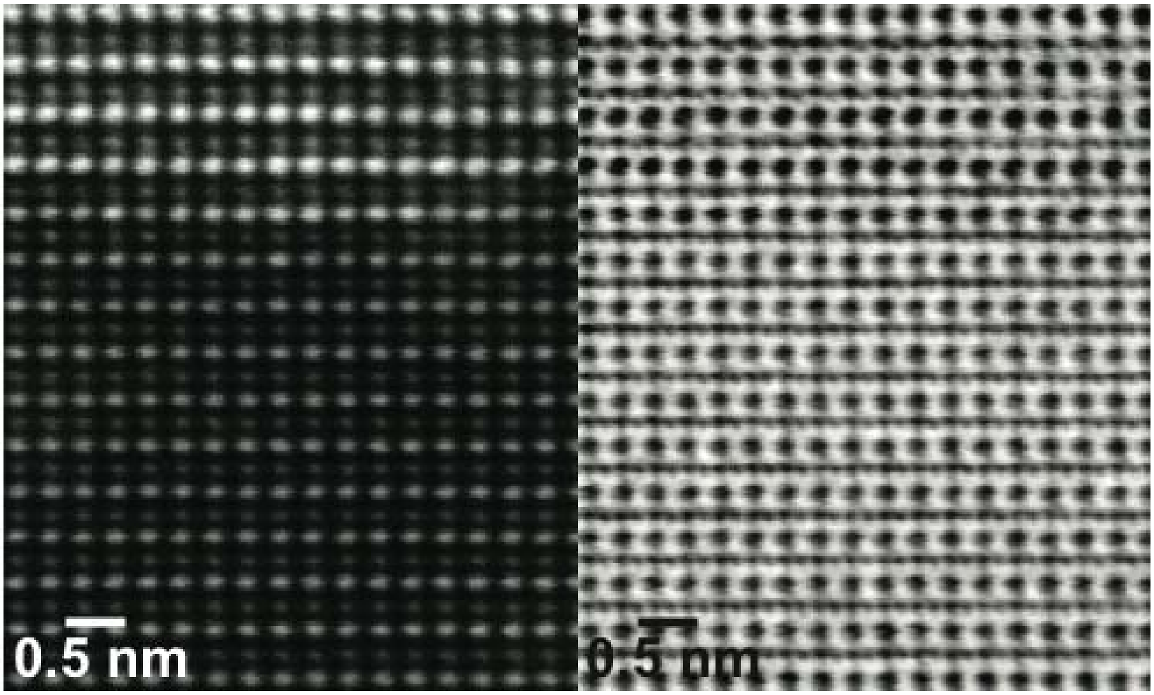


Fig. S1 Simultaneously collected ADF (left) and BF (right) image of the PZT/STO interface as viewed along the <110> direction.

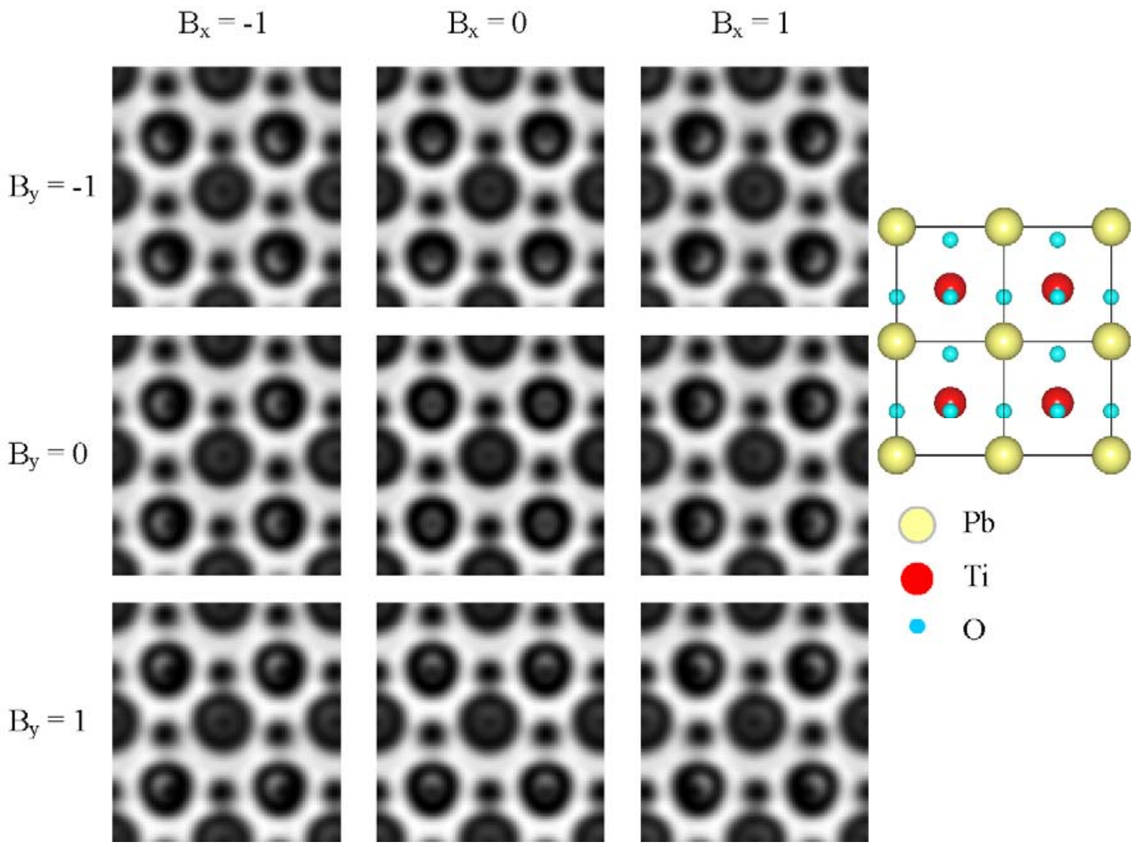


Fig. S2. STEM BF image simulations of PTO in the [100] zone axis orientation as a function of crystal tilt in units of Bragg angles. $B_x = 1$ corresponds to the component of the incident beam tangential to the crystal surface being $k_t = -[010]/2$. $B_y = 1$ corresponds to $k_t = -[001]/2$. The projected structure is shown to the right.

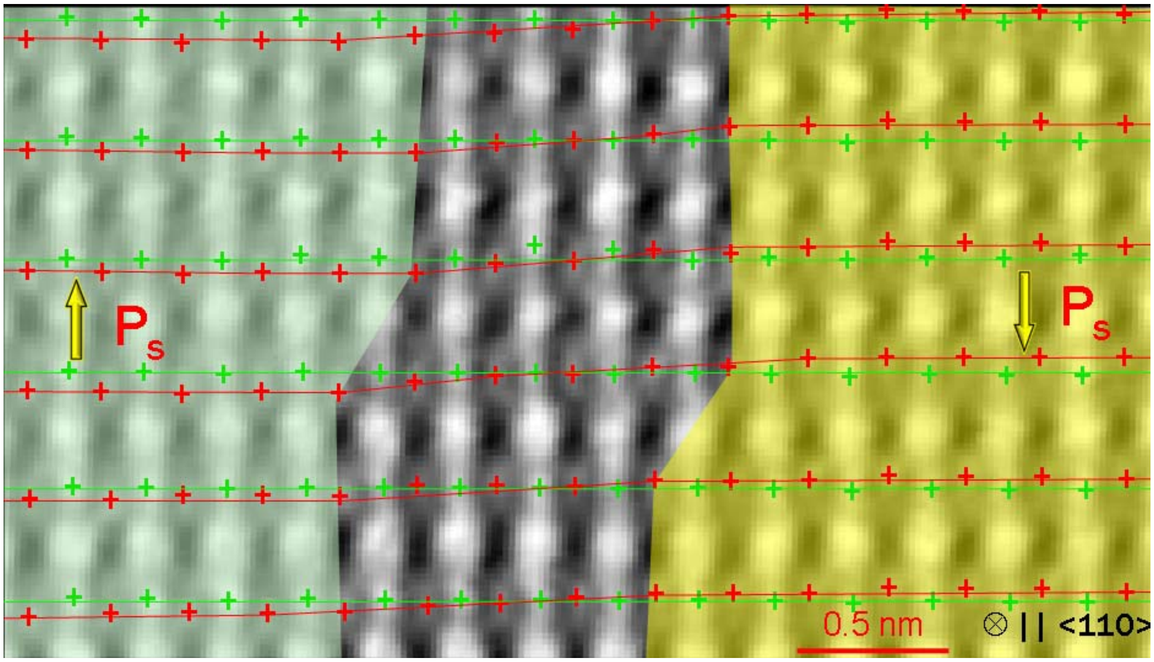


Fig. S3 Phase contrast image of a ferroelectric domain wall in PZT in the <110> projection. Marking the oxygen column positions in red and the titanium column positions in green, the two 180˚ domains and a 1 nm thick domain wall can be seen.

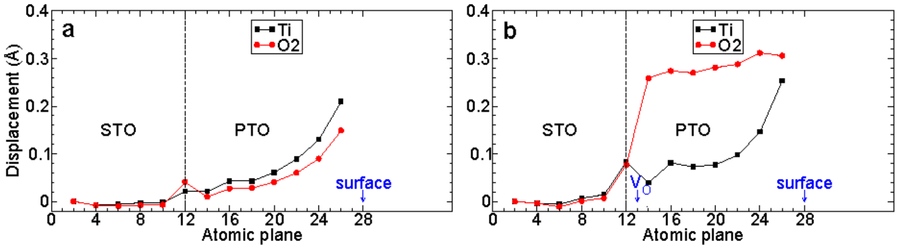


Fig. S4. Calculated ferroelectric displacements at the STO/PTO interfaces with PTO free surface. (a), The ferroelectric displacements are severely suppressed at the perfect interface.(b), The ferroelectric displacements in PTO recover to values close to bulk with the presence of one O vacancy for every four interfacial units, in agreement with experimental observations.
